# Supplementary material for: Dynamics of Motility-Induced clusters: coarsening beyond Ostwald ripening
Source: arXiv:2211.12361 source file (2022-11-22)
Supplement: Supplementary file 1 [file timetracking.tex]

\vspace{0.25cm}

\section{Time tracking for clusters in the bulk}
\label{sec:timetracking}

In order to study more in depth the mechanism of clusters growing, we have developed an algorithm for clusters tracking over time.
Given the state of the system at a give time, we group particles into separate clusters and the gaseous background by means of the the DBSCAN algorithm.
We then compare two configurations at two successive times $t$ and $t+\Delta t$, respectively, and we establish a correspondence between clusters, based on a computation of the overlap between them.
The normalised overlap between cluster $i$ at time $t$ and cluster $j$ at time $t+\Delta t$ is measured as
\begin{equation}
  o_{ij}=\frac{n_{ij}}{\sqrt(M_i M_j)} \mbox{,}
\end{equation}
where $n_{ij}$ is the number of particles belonging to both clusters and $M_i$, $M_j$ the masses of the two clusters, respectively.
The overlap is computed for any $i=1,...,N_t$ and $j=1,...,N_{t+\Delta t}$.

Then, an upper threshold $T_u$ and a lower one $T_l$ for the overlap are introduced, in order to identify different types of collisional events, occurring within the time interval $\Delta t$, according to the following criteria:
\begin{itemize}
\item if $o_{ij}>T_u$, then cluster $i$ has evolved without collisions with other clusters, and it has become cluster $j$ at time $t+\Delta t$;
\item if $o_{ij}<T_u$ for any $j=1,...,N_{t+\Delta t}$ and $\sum_{j=1}^{N_{t+\Delta t}} o_{ij}>T_u$, then cluster $i$ has broken into pieces. The residual clusters after the breaking are the ones such that $o_{ij}>T_l$;
\item if $o_{ij}<T_u$ for any $i=1,...,N_t$ and $\sum_{i=1}^{N_t} o_{ij}>T_u$, then several clusters have coalesced into cluster $j$. The clusters that have contributed to the coalescence are the ones such that $o_{ij}>T_l$.
\end{itemize}

The presence of these thresholds allows us to distinguish between events involving a relatively small number of particles, which we associate with Ostwald ripening mechanism, and events involving collisions between macroscopic clusters.
We use $\Delta t=10$ as a fixed time separation between two consecutive configurations of the system.
{\textcolor{blue}{*** We actually use always $10^4$ timesteps for both $Pe=0$ and $Pe=100$, but the timestep for $Pe=0$ is $5$ times longer. The ideal would be to have $Pe=0$ sampled every $2000$ steps, in order to have the same $\Delta t$ for both and a not too long $\Delta t$ for $Pe=100$. ***}}
The values $T_u=0.9$ and $T_l=0.1$ are chosen, so that mass variations smaller than $\Delta M\simeq100$ are identified as a Ostwald ripening evaporation-condensation process, while larger mass variations are identified as collisions between clusters.

We show in Fig.\ref{fig:collision_table} an illustrative representation of the result of the tracking.

\begin{figure}
\label{fig:collision_table}
\centering
\includegraphic[width=\textwidth]{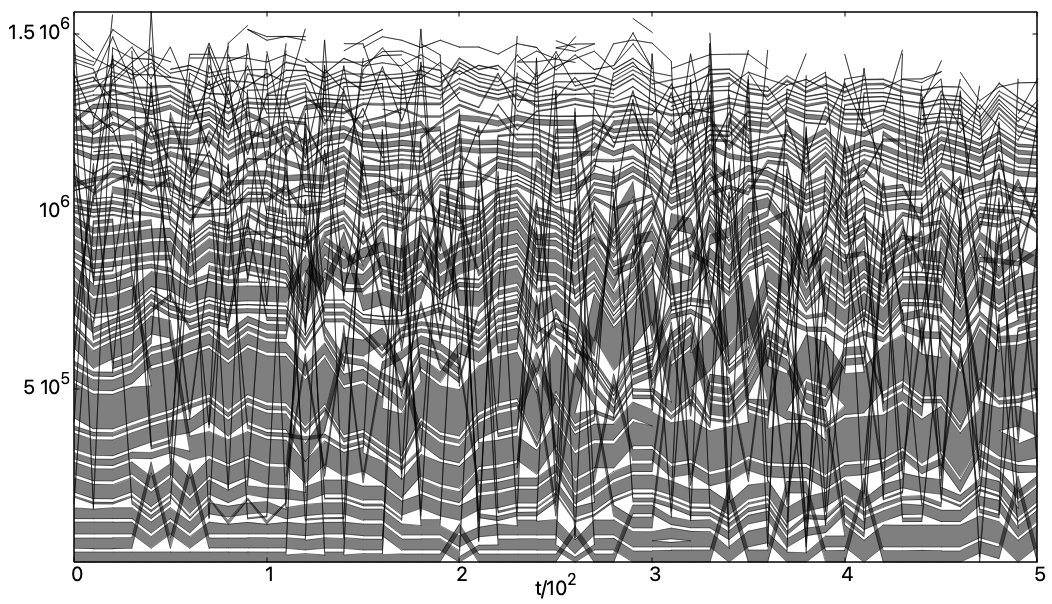}
\caption{Clusters tracks, as extracted with the algorithm described in the text. At a given time, each grey band corresponds to one cluster. The width of the bands is equal to the cluster's mass. Moving from one time to the next one, two or bands can merge into one, which corresponds to a coalescence event, or one band can divide into several ones, which corresponds to a breaking event. The cases where the band remains isolated correspond to a cluster evolving isolated from the others. Within these time windows, the clusters gains or loses mass through evaporation or condensation of a small number of particles. See the text for a detailed description of these processes.}
\end{figure}
